# Supplementary material for: Multi-Agent Resilient Consensus under Intermittent Faulty and Malicious Transmissions (Extended Version)
Source: arXiv:2403.17907 source file (2024-03-26)
Supplement: Supplementary file 1 [file appendix.tex]

% !TEX root = Control of stochastic disease network games via influential individuals.tex

\section{Appendix}
\label{sec:app}
%\vspace{-5pt}

\subsection{Proof of Lemma \ref{lem_pg_def}}
\label{sec_app_pg_proof}
We use  Policy Gradient Theorem \cite{sutton1999policy}, to define the policy as below,
\begin{align}
    \nabla_i u_i(\theta_i,\theta_{-i})&=\int_{\substack{a \in \mathcal{A},\\ s \in \mathcal{S}}} Q_i^{\Pi_\theta} (s,a) d^{\Pi_\theta}  \nabla_i\pi_\theta(a|s) \, da \, ds,
 \end{align}   
where $d^{\Pi_\theta}=\sum_{t=0}^\infty \gamma^{t} \rho_{s_0,s,t}^{a}$ is the discounted sum of density functions $\rho_{s_0,s,t}^{a}$ of the transition probability function $\ccalP_{s_0,s,t}^{a}$ from the initial state $s_0$ to the state $s$ giventhe joint action profiles from time $t=0$ to $t=\infty$, $a_{0:t}$, and similarly $\pi_\theta(a|s)$ is defined as the density function of the joint policy $\Pi_\theta$ parameterized by $\theta$. 

Then, applying the log-likelihood transformation by dividing and again multiplying the gradient of $\nabla_i\pi_\theta(a|s)$ by the density $ \pi_\theta(a|s)$, we obtain the following, 

 \begin{align}   
     \nabla_i u_i&(\theta_i,\theta_{-i})\hspace{-2pt}=\hspace{-2pt}\int_{\substack{a \in \mathcal{A},\\ s \in \mathcal{S}}} Q_i^{\Pi_\theta}(s,a) d^{\Pi_\theta}  \pi_\theta(a|s)  \frac{\nabla_i\pi_\theta(a|s)}{\pi_\theta(a|s)}  \, da \, ds\\
    &=\int_{\substack{a \in \mathcal{A},\\ s \in \mathcal{S}}} Q_i^{\Pi_\theta}(s,a)d^{\Pi_\theta}  \pi_\theta(a|s) \nabla_i \log \pi_\theta(a|s) \, da \, ds.
    \end{align}
We divide the integral by $(1-\gamma)$ to have a expectation defined over a probability distribution, and use the definition in \eqref{eq_ind_pol}, 
 such that the policy gradient becomes,
    \begin{align}
    &=\int_{\substack{a \in \mathcal{A},\\ s \in \mathcal{S}}} Q_i^{\Pi_\theta} (s,a) d^{\Pi_\theta}  \pi^\theta(a|s) \sum_{n \in \ccalN} \nabla_i \log \pi_{n,\theta}(a_n|s)  \, da \, ds\\
    %&=\int_{a_i \in \mathcal{A}_i, s\in \mathcal{S}} d^{\Pi_\theta} \pi_i^\theta(a_i|s) \nabla_i \log \pi^\theta(a_i|s) \\
    %&\Big (\int_{a_{-i} \in \mathcal{A}^{N-1}} Q_i^{\Pi_\theta} (s,a)(1-\gamma)\pi_{-i}^\theta(a_{-i}|s)da_{-i}\Big)  \, da_i \, ds \nonumber \\
    & = \frac{1}{(1-\gamma)} \: \mathbb{E}_{(s,a) \sim \ccalP}\big[Q_i^{\Pi_\theta} (s,a)\sum_{n \in \ccalN} \nabla_i \log \pi_{n,\theta}(a_n|s) \big].
\end{align}

\subsection{Proof of Lemma \ref{lemma_lip}} \label{app_lem2}

\begin{comment}
 \begin{lemma}[Lipschitz-Continuity of Policy Gradients] \label{lemma_lip}   
Suppose Assumption \ref{as_bound_logp} holds. The policy gradient of any agent $i\in \ccalN$,  $\nabla_{i} u_{i} (\theta_{i}, \theta_{-i})$ is Lipschitz continuous with some constant $L_2>0,$ i.e., for any $\theta_{i}^{1}, \theta_{i}^{2} \in \mathbb{R}^{M}$
\begin{equation}
 ||\nabla_{i} u_{i} (\theta_{i}^1, \theta_{-i}^1) -\nabla_{i} u_{i} (\theta_{i}^{2}, \theta_{-i}^{2})|| \le L ||\theta^{1} -\theta^{2}||,
\end{equation}where the value of the Lipschitz constant $L$ is defined as 
\begin{equation}\label{eq_lip_const}
L:= N R(\frac{1}{(1-\gamma^2)} \red{\ccalL} +\frac{(1+\gamma)}{(1-\gamma)^3 B^2} ).
\end{equation}
\end{lemma}
\end{comment}

Using the definition of policy gradients, we firstly re-expand the definition of discounted state-action distribution. We then substitute the order of integral and summations by Fubini's Theorem as the result of Assumptions \ref{as_bound_rew}-\ref{as_bound_logp} so that the individual stochastic gradients are always bounded and therefore the expectation (first moment) of the gradients is always bounded,
%\blue{CE: You need the left hand side of this equality, i.e., the policy gradient here...}
\begin{align}
%\ccalP_{s_0,s,t}^{\pi^\theta} \pi^\theta(a_t|s_t)
&\nabla_i u_i(\theta_i,\theta_{-i})\\
&=\int_{\substack{a \in \mathcal{A}^N,\\s \in \mathcal{S}}} d^{\Pi_\theta}  \pi_\theta(a|s) \bigg(\sum_{n \in \ccalN} \nabla_i \log \pi_{n,\theta}(a_n|s)\bigg) Q_i^{\Pi_\theta} (s,a) \, da \, ds  \\
=&\sum_{n \in \ccalN} \sum_{t=0}^\infty \sum_{\tau=0}^\infty \gamma^{t+\tau}\int_{\substack{a_{t} \in \mathcal{A},\\ s_{t}\in \mathcal{S}}}  r_{it}(s_{t+\tau},a_{t+\tau})\nabla_i \log \pi_{n,\theta}(a_{n,t}|s_t)   \nonumber\\ &  \hspace{105pt} \rho^{\theta}_{t+\tau} \, da_{0:t+\tau} \, ds_{1:t+\tau} \label{eq_pg_def_lip}
\end{align}
where $\rho^{\theta}_{t+\tau}= \prod_{h=0}^{t+\tau-1} \ccalP^{a_h}_{s_h,s_{h+1}} \prod_{h=0}^{t+\tau} \pi_\theta(a_{h}|s_h)$ is defined as the result of Markovian state-action sequence. We now express the norm of the difference between the gradients defined at any two points $\theta^1,\theta^2 \in \reals^M$ as per \eqref{eq_pg_def_lip},
 
 \begin{align}
&|| \nabla_{i} u_{i} (\theta_{i}^1, \theta_{-i}^1) -\nabla_{i} u_{i} (\theta_{i}^{2}, \theta_{-i}^{2})|| \\
& = || \sum_{n \in \ccalN} \sum_{t=0}^\infty \sum_{\tau=0}^\infty \gamma^{t+\tau} ( \int_{\substack{a_{t} \in \mathcal{A},\\ s_{t}\in \mathcal{S}}}  r_{it}(s_{t+\tau},a_{t+\tau})\nonumber\\ &  (\nabla_i \log \pi_{n,\theta_1}(a_t|s_t) - \nabla_i \log \pi_{n,\theta_2}(a_t|s_t))  \rho^{\theta_1}_{t+\tau}  da_{0:t+\tau} \, ds_{1:t+\tau})  \nonumber\\
&+(\int_{\substack{a_{t} \in \mathcal{A},\\ s_{t}\in \mathcal{S}}}  r_{it}(s_{t+\tau},a_{t+\tau})\nabla_i \log \pi_{n,\theta_2}(a_t|s_t)(\rho^{\theta_1}_{t+\tau}-\rho^{\theta_2}_{t+\tau})) \nonumber\\
 &da_{0:t+\tau} \, ds_{1:t+\tau}) || \label{eq_Lip_norm_def}. 
 %&\int_{\substack{a_{t} \in \mathcal{A},\\ s_{t}\in \mathcal{S}}}  r_{it}(s_{t+\tau},a_{t+\tau})  (\nabla_i \log \pi_n^{\theta_1}(a_t|s_t) - \nabla_i \log \pi_n^{\theta_2}(a_t|s_t))  \rho^{\theta_1}_{t+\tau}  da_{0:t+\tau} \, ds_{1:t+\tau})
 \end{align}
 %\blue{CE: Clarify the simple algebraic modification you have here to get (56)...}
 We show Lipschitz continuity separately for each integral inside the nested sum. Using triangle inequality, the first integral is bounded by Assumptions \ref{as_bound_rew}-\ref{as_bound_logp}
 \begin{align}
 & ||\int_{\substack{a_{t} \in \mathcal{A},\\ s_{t}\in \mathcal{S}}}  r_{it}(s_{t+\tau},a_{t+\tau})\nonumber\\ 
 &  (\nabla_i \log \pi_{n,\theta_1}(a_t|s_t) - \nabla_i \log \pi_{n,\theta_2}(a_t|s_t))  \rho^{\theta_1}_{t+\tau}  da_{0:t+\tau} \, ds_{1:t+\tau} ||\\
     &\le \int_{\substack{a_{t} \in \mathcal{A},\\ s_{t}\in \mathcal{S}}}  |r_{it}(s_{t+\tau},a_{t+\tau})| \: ||\nabla_i \log \pi_{n,\theta_1}(a_t|s_t)\\
     &- \nabla_i \log \pi_{n,\theta_2}(a_t|s_t)|| \nonumber  
    \rho^{\theta_1}_{t+\tau}  da_{0:t+\tau} \, ds_{1:t+\tau} \le R \ccalL || \theta^1-\theta^2|| \label{eq_bound_I1}.
 \end{align}
 
Next, we show Lipschitz continuity of the second integral, by defining the difference in probability measures as the product of state transitions and policies,

\begin{align}
    &\rho^{\theta_1}_{t+\tau}-\rho^{\theta_2}_{t+\tau}\\ 
    &= \prod_{h=0}^{t+\tau-1} \ccalP^{a_h}_{s_h,s_{h+1}} (\prod_{h=0}^{t+\tau} \pi_{n,\theta_{1}} (a_{n,h}|s_h) -\prod_{m=0}^{t+\tau} \pi_{n,\theta_{2}} (a_{n,h}|s_h)).
\end{align}

We bound the difference between two policies parametrized by $\theta^1,\theta^2 \in \reals^M$ with Taylor expansion,
\begin{align}
    &P_2=|\prod_{h=0}^{t+\tau} \pi_{n,\theta_{1}}(a_{n,h}|s_h) -\prod_{m=0}^{t+\tau} \pi_{n,\theta_{2}} (a_{n,h}|s_h)| \label{eq_pol_dif}\\
    & \le | (\theta^1-\theta^2)^T(\sum_{h'=0}^{t+\tau} \nabla_i \pi_{n,\Tilde{\theta}}(a_{n,h'}|s_{h'}) \prod^{t+\tau}_{\substack{h=0\\ h \neq h'}} \pi_{n,\Tilde{\theta}} (a_{n,h}|s_h)|,
\end{align}
where $\Tilde{\theta}=\varrho \theta^1+(1-\varrho)\theta^2$ is a convex combination of the points (vectors) $\theta^1,\theta^2 \in \reals^M$ for some $\varrho \in [0,1]$. The upper bound again follows from triangle inequality, 

\begin{align}
    & \le || \theta^1-\theta^2|| \sum_{h'=0}^{t+\tau} || \nabla_i \log \pi_{n,\Tilde{\theta}} (a_{n,h'}|s_{h'})|| \prod^{t+\tau}_{h=0}||\pi_{n,\Tilde{\theta}} (a_{n,h}|s_h)||\\
    & \le || \theta^1-\theta^2|| (t+\tau+1) B\prod^{t+\tau}_{h=0}\pi_{n,\Tilde{\theta}} (a_{n,h}|s_h). \label{eq_up_bound_pol}
    %&\le  || \theta^1-\theta^2|| (t+\tau+1) B 
\end{align}
where the term $\prod^{t+\tau}_{h=0}\pi_{n,\Tilde{\theta}} (a_{n,h}|s_h)$ is a product of proper probability densities. Inserting \eqref{eq_up_bound_pol} into the second integral in \eqref{eq_Lip_norm_def} gives, %\blue{CE: again confusing without the left hand side...Are you bounding (56) or just the second integral in (56)?}
%\begin{comment}
\begin{align}
    %&||\int_{\substack{a_{t} \in \mathcal{A},\\ s_{t}\in \mathcal{S}}}  r_{it}(s_{t+\tau},a_{t+\tau})\nabla_i \log \pi_n^{\theta_2}(a_t|s_t) \nonumber\\&(\rho^{\theta_1}_{t+\tau}-\rho^{\theta_2}_{t+\tau}) da_{0:t+\tau} \, ds_{1:t+\tau}||\\
    %&\le \int_{\substack{a_{t} \in \mathcal{A},\\ s_{t}\in \mathcal{S}}}  |r_{it}(s_{t+\tau},a_{t+\tau})| ||\nabla_i \log \pi_n^{\theta_2}(a_t|s_t)|\rho^{\theta_1}_{t+\tau}-\rho^{\theta_2}_{t+\tau}| da_{0:t+\tau} \, ds_{1:t+\tau}\\
    & P_2\le \int R B || \theta^1-\theta^2|| (t+\tau+1) B\prod^{t+\tau}_{h=0}\pi_{n,\Tilde{\theta}} (a_{n,h}|s_h) \nonumber\\
     &\times \prod_{h=0}^{t+\tau-1} \ccalP^{a_h}_{s_h,s_{h+1}}da_{0:t+\tau} \, ds_{1:t+\tau} \\
    & \le  || \theta^1-\theta^2|| (t+\tau+1)  R B^2 \label{eq_bound_I2}.
\end{align}
Thus, combining the bounds \eqref{eq_bound_I1} and \eqref{eq_bound_I2} on the integrals concludes the Lipschitz continuity as follows,
\begin{align}
    &||\nabla_{i} u_{i} (\theta_{i}^1, \theta_{-i}^1) -\nabla_{i} u_{i} (\theta_{i}^{2}, \theta_{-i}^{2})||   \\
    &\le \sum_{n \in \ccalN} \sum_{t=0}^\infty \sum_{\tau=0}^\infty \gamma^{t+\tau} R \bigg( \ccalL +B^2 (t+\tau+1)\bigg) || \theta^1-\theta^2|| \\
    & \le N R\bigg(\frac{1}{(1-\gamma^2)} \ccalL +\frac{(1+\gamma)B^2}{(1-\gamma)^3} \bigg) || \theta^1-\theta^2||.
\end{align}
\subsection{Proof of Lemma \ref{lem_unb}}
\label{sec_app_lem_unb}

We bound the norm of the stochastic policy gradients by Assumptions \ref{as_bound_rew}-\ref{as_bound_logp}, 
%\blue{CE: I do not follow why 79 is  a bound on 78. Aren't they equal? Also can't you begin with (79) here? (79) is how you define gradient in eq. (7)...}

\begin{align}
 &|| \hat{\nabla}_i u_i(\theta_i,\theta_{-i})|| =\frac{1}{(1-\gamma)} || \hat{Q}_i^{\Pi_{\theta}} \sum _{n \in \ccalN} \nabla_i \log \pi_{n,\theta}(a_{n,\ccalT_1}|s_{\ccalT_1}) || \\
 & \le \frac{1}{(1-\gamma)} N B || \hat{Q}_i^{\Pi_{\theta}}|| \le  \frac{1}{(1-\gamma)} N B \sum_{\tau=1}^{\ccalT_2} \gamma^{1/2} r_{i,\tau} (s_\tau,a_\tau)
 \end{align}
 %\blue{CE: Assumption 6 says $||\nabla_i \log \pi_{i,\theta} (a_i| s)|| \le B$. But what about $||\nabla_i \log \pi_{n,\theta} (a_n| s)||$  }
We extend the sum of the rewards through infinity to obtain the geometric sum and again use the upper bound on the rewards by Assumption \ref{as_bound_rew},
 \begin{align}
 & \le  \frac{N B }{(1-\gamma)} \sum_{\tau=1}^\infty \gamma^{1/2} r_{i,\tau} (s_\tau,a_\tau) \le  \frac{NB}{(1-\gamma)}\sum_{\tau=1}^\infty \gamma^{1/2} R \\
 &\le \frac{ N B R}{(1-\gamma) (1-\gamma^{1/2})} 
\end{align}
%\blue{CE: New paragraph here. You are starting something new...}
%\blue{CE: What are these horizons? Tell it here...} 
We state the expectation of the stochastic policy gradient, by taking expectations over the wo different horizons $\ccalT_1$ and $\ccalT_2$ and the distribution of state-action pairs observed through these horizons consecutively, 
\begin{align}
&\mathbb{E}[\hat{\nabla}_i u_i(\theta_i,\theta_{-i})|\theta]\\
=&\mathbb{E}_{\substack{\ccalT_1, s_{\ccalT_1},\\ a_{\ccalT_1}}}[\mathbb{E}_{\substack{\ccalT_2,s_{1:\ccalT_2},\\ a_{1:\ccalT_2} }}[\hat{\nabla}_i u_i(\theta_i,\theta_{-i})|s_{\ccalT_1}, a_{\ccalT_1},\theta] |\theta]
\end{align}
We indicate the value of the inner expectation using Lemma \ref{lem_q_unb} and the fact that the gradient of log-policy is independent of the given variables $\ccalT_2,s_{1:\ccalT_2}$ and $ a_{1:\ccalT_2}$,
\begin{align}
=&\mathbb{E}_{\substack{\ccalT_1, s_{\ccalT_1},\\ a_{i,\ccalT_1}}}\bigg[\mathbb{E}_{\substack{\ccalT_2,s_{1:\ccalT_2},\\a_{i,1:\ccalT_2} }}\big[\frac{1}{1-\gamma}\hat{Q}_i^{\Pi_{\theta}}( s_{\ccalT_1}, a_{\ccalT_1})\nonumber \\ 
& \times \nabla_i \log \pi_\theta(a_{\ccalT_1}|s_{\ccalT_1})| s_{\ccalT_1}, a_{\ccalT_1}, \theta\big]|\theta\bigg]\\
=&\mathbb{E}_{\substack{\ccalT_1, s_{\ccalT_1},\\ a_{\ccalT_1}}}\bigg[\frac{1}{1-\gamma}Q_i^{\Pi_{\theta}}(s,a)\nabla_i \log \pi_\theta(a|s)|\theta\bigg]\label{eq_outer_exp}
\end{align}
%\blue{CE: You moved from $\hat Q$ to $Q$... How? explain?}
where we obtained the unbiased estimation of $Q$-values by independently sampled horizons. 
Since the norm of the gradient estimate is always bounded with the term for any state and action pair of $(s,a) \in \ccalS \times \ccalA^N$, its expectation is also bounded. We  further rewrite \eqref{eq_outer_exp} using indicator variables, and then by Fubini's Theorem, we take the summation over the infinite horizon out of the expectation,
\begin{align}
    =&\mathbb{E}_{\ccalT_1,s_{\ccalT_1}, a_{\ccalT_1}}\bigg[\sum_{t=0}^{\infty}\mathbb{1}_{ t = \ccalT_1} \frac{1}{1-\gamma}Q_i^{\Pi_{\theta}}(s,a)\log \pi^\theta(a|s)|\theta\bigg], \\
    =&\frac{1}{1-\gamma} \sum_{t=0}^{\infty}\mathbb{P}( t = \ccalT_1)\mathbb{E}_{s_{\ccalT_1}, a_{\ccalT_1}}[ Q_i^{\Pi_{\theta}}(s,a)\log \pi_\theta(a|s)|\theta],\\
    =&\sum_{t=0}^{\infty}\gamma^t \mathbb{E}_{s_{\ccalT_1}, a_{\ccalT_1}}[Q_i^{\Pi_{\theta}}(s,a)\log \pi_\theta(a|s)|\theta]
\end{align}
%\blue{Explain the last equality? In particular, what happened to $P(t=\ccalT_1)$?}
where we use the equality $P(\ccalT_1=t)=\gamma^{t/2}$
Next, we apply the definition of expectation with respect to the given distribution,

\begin{align}
    =&\sum_{t=0}^{\infty}\gamma^t \int_{\substack{a \in \mathcal{A},\\ s \in \mathcal{S}}} \frac{1}{(1-\gamma)} Q_i^{\Pi_{\theta}}(s,a)\log \pi_\theta(a|s) \ccalP_{s,s',t}^{\pi_\theta} ds da,\\
    =&\int_{\substack{a \in \mathcal{A},\\ s \in \mathcal{S}}} \frac{1}{(1-\gamma)}\sum_{t=0}^{\infty}\gamma^t   Q_i^{\Pi_{\theta}}(s,a)\log \pi_\theta(a|s) \ccalP_{s,s',t}^{\pi_\theta} dsda.
\end{align}

Thus, we recover the definition of policy gradients by the fact  $d^{\Pi_\theta}(s)=\sum_{t=0}^\infty \gamma^{t} \ccalP_{s_0,s,t}^{\pi^\theta} $, and conclude that the stochastic gradient is unbiased,

\begin{equation}
   =\int_{\substack{a \in \mathcal{A},\\ s \in \mathcal{S}}} \frac{1}{(1-\gamma)} d^{\Pi_\theta}(s) Q_i^{\Pi_{\theta}}(s,a)\log \pi_\theta(a|s) ds da.
\end{equation}

 \subsection{Unbiasedness of $\hat{Q}$}

 \begin{lemma} \label{lem_q_unb}
 The estimates $\hat{Q}_i^{\Pi_{\theta}}$ for each agent $i \in \ccalN$ computed by Algorithm \ref{alg_DFP} is unbiased, $\mathbb{E}[\hat{Q}_i^{\Pi_{\theta}} (s,a)| s_0=s, a_{0}=a, \theta]=Q_i^{\Pi_{\theta}} (s,a)$.
 \end{lemma}
 %and $\hat{V}_i^{\Pi_{\theta}}(s)$  of o
 %and $\mathbb{E}(\hat{V}_i^{\Pi_{\theta}} (s)| s_0=s, \theta)=V_i^{\Pi_{\theta}} (s)$
 \begin{proof} 
 Using the definition of $\hat{Q}_i$, we transform the finite sum of rewards over the sampled horizon length into an infinite sum,
 \begin{align}
 &\mathbb{E}[\hat{Q}_i^{\Pi_{\theta}} (s,a)| s_0=s, a_{0}=a, \theta]\\
 = &\mathbb{E}[\sum_{t=0}^{\ccalT_2} \gamma^{t/2} r_{it}(s_t,a_t) | s_0=s, a_{0}=a, \theta]\\
 =&\mathbb{E}[\sum_{t=0}^{\infty} \mathbb{1}_{(1\le t \le \ccalT_2)} \gamma^{t/2} r_{it}(s_t,a_t) | s_0=s, a_{0}=a, \theta]\label{eq_est_def}.
 \end{align}
 %\vspace{-0.05 in}
%where $\sum_{t=0}^{\infty} \mathbb{1}_{(1\le t \le \ccalT_2)} \gamma^{t/2} r_{it}(s_t,a_t)= \lim_{\ccalT \xrightarrow{} \infty} \sum_{t=0}^{\ccalT} \mathbb{1}_{(1\le t \le \ccalT_2)} \gamma^{t/2} r_{it}(s_t,a_t)$. 
The absolute value of function sequence satisfies, $ |\sum_{t=0}^{\ccalT} \mathbb{1}_{(1\le t \le \ccalT_2)} \gamma^{t/2} r_{it}(s_t,a_t)| \le  \sum_{t=0}^{\ccalT} \gamma^{t/2} R$ by Assumption \ref{as_bound_rew}.  Then, since $\lim_{\ccalT \xrightarrow{} \infty} \sum_{t=0}^{\ccalT} \mathbb{E}( \gamma^{t/2} R)=\sum_{t=0}^{\infty} \gamma^{t/2} R < \infty$ exists and, is integrable, given $\gamma \in (0,1)$. Therefore, we rewrite \eqref{eq_est_def} with General Lebesgue Dominated Convergence Theorem,
 
\begin{align}
   &\mathbb{E}[\sum_{t=0}^{\infty} \mathbb{1}_{(1\le t \le \ccalT_2)} \gamma^{t/2} r_{it}(s_t,a_t) | s_0=s, a_{0}=a, \theta] \\
 =&\sum_{t=0}^{\infty}\mathbb{E}[\mathbb{1}_{(1\le t \le \ccalT_2)} \gamma^{t/2} r_{it}(s_t,a_t) | s_0=s, a_{0}=a, \theta]
 \end{align}
The randomness stems from the stochastic joint policy and state transition together with the sampled horizon length. Then, we split the expectation of discounted state-action distribution and the distribution of random horizon lengths,
 \begin{align}
 =&\sum_{t=0}^{\infty}\mathbb{E}_{(s,a)}[\mathbb{E}_{\ccalT_2}(\mathbb{1}_{(1\le t \le \ccalT_2)}) \gamma^{t/2} r_{it}(s_t,a_t) | s_0=s, a_{0}=a, \theta]\\
 =&\sum_{t=0}^{\infty}\mathbb{E}_{(s,a)}[\gamma^{t} r_{it}(s_t,a_t) | s_0=s, a_{0}=a, \theta]
\end{align}
%\blue{CE: point out that you are using the fact that $\ccalT_2$ is Geometric with $(1-\gamma^{0.5}$...}
where we take expectation over the random variable $\ccalT_2 \sim Geom(1-\gamma^{0.5})$.
Again by General Lebesgue Dominated Convergence Theorem, we exchange the order of the expectation operator and summation to show the unbiasedness,

\begin{align}
    %&\sum_{t=0}^{\infty}\mathbb{E}_{(s,a)}(\gamma^{t} r_{it}(s_t,a_t) | s_0=s, a_{0}=a, \theta)\\
    &= \mathbb{E}_{(s,a)}[\sum_{t=0}^{\infty}\gamma^{t} r_{it}(s_t,a_t) | s_0=s, a_{0}=a, \theta]= Q_i^{\Pi_{\theta}} (s,a).
\end{align}

\begin{comment}
Following the same way of analysis, we can show unbiased estimate of value function of agent $i$ such that,
\begin{align}
&\mathbb{E}(\sum_{t=0}^{\infty} \mathbb{1}_{(1\le t \le \ccalT_2)} \gamma^{(t/2)} r_{it}(s_t,a_t) | s_0=s, \theta)\\
&=\mathbb{E}(\hat{V}_i^{\Pi_{\theta}}(s) | s_0=s, \theta) =V_i^{\Pi_{\theta}}(s).
\end{align}
\end{comment}

 \end{proof}
